# Supplementary material for: MoRE: Multi-Modal Contrastive Pre-training with Transformers on X-Rays, ECGs, and Diagnostic Report
Source: arXiv:2410.16239 source file (2024-10-22)
Supplement: Supplementary file 1 [file appendix_auc.tex]

\section*{Appendix C. X-ray Inference Results (AUC) in 10\%  and 50\%data}
\label{appendix:results_auc_10_50}
\begin{table}[H]
\centering
\begin{tabular}{l|c|c|c|c|c|c|c|c}
\multicolumn{9}{c}{AUROC on 10 \% Data} \\
\hline
\multirow{2}{*}{Model} & \multicolumn{4}{c}{Mimic IV} & \multicolumn{4}{c}{Chexpert} \\
\cline{2-9} 
& AC & CM & ED & PE & AC & CM & ED & PE \\
\hline
Gloria &\bf0.74& 0.73& 0.81 &0.83 &0.76 & 0.77 & 0.87 & \bf0.90 \\
\hline
MedKlip & 0.69&0.65 & 0.76& 0.82& 0.75& 0.76& \bf0.91& \bf0.90 \\
\hline
\tool\ &\bf0.74 &\bf0.78 &\bf0.83 &\bf 0.86 &0.71 &\bf0.78 &0.89 &0.88 \\
% Add more models as needed
\hline
\\
\multicolumn{9}{c}{AUROC on 50 \% Data} \\
\hline
& AC & CM & ED & PE & AC & CM & ED & PE \\
\hline
Gloria &0.75 &0.75 &0.81 &0.86 & 0.76 & 0.77 & 0.87 & 0.90 \\
\hline
MedKlip & 0.71& 0.66& 0.76& 0.82& 0.73& 0.77& \bf0.91& \bf0.91 \\
\hline
\tool\ &\bf0.80 &\bf0.83 &\bf0.89 &\bf0.89 &0.71 & \bf0.81 & 0.90 & 0.90 \\
\hline
\\
\end{tabular}
\caption{X-ray Inference Results (AUC) in 10\% and 50\% data}
\label{xray-auc}
\end{table}
